# Supplementary material for: Protecting against simultaneous data poisoning attacks
Source: arXiv:2408.13221 source file (2024-08-23)
Supplement: Supplementary file 1 [file appendix.tex]

\appendix

\section{Appendix}

\subsection{Algorithm}
\label{sec:algorithm}

Notation: Dataset $D$, potentially backdoored. Subset $C \in D$ of $2n$ bona-fide clean examples. Learning algorithm that takes a dataset $D$ and produces a learned $M$ and a time series of losses $L$ for each data point in the given dataset: $\mathcal{A}: D \rightarrow M, L$.  Parameters $k \in \mathbb{N}$, $t \in [0, 1]$. A reference backdoor function $B: D \rightarrow D$ that takes datapoints in $D$ and adds a backdoor to them, possibly changing their labels.

\begin{enumerate}
    \item Select half of the clean examples ($n$ examples) in $C$ as $P_1$. These examples will stay clean.
    \item Select the remaining $n$ clean examples in $C$ and use $B$ to add a backdoor to them, producing $P_2$
    \item Select $n$ additional examples from the dataset $D$ and randomize their labels so that every example is mislabeled -- call this set of points $P_3$.
    \item Inject $P_1, P_2, P_3$ into $D$, overwriting their previous points. Call this dataset $D'$
    \item Train a model $M'$ on $D'$ using $\mathcal{A}$, producing a series of training losses $L$. $L$ contains a loss trajectory per example, where each loss trajectory is a sequence of real numbers of length equal to the number of epochs of training. 
    \item Select the losses for $P_1$, $P_2$, and $P_3$, treating the losses as Euclidean vectors. Call these losses the probe set. $P_1$ is the clean probe set, $P_2$ and $P_3$ are the anomalous probe set.
    \item For each training examples in $D' \not\in P_1 \cup P_2 \cup P_3$, find the $k$ nearest neighbors in the probe set, using Euclidean distance. If more than $t$ of the neighbors are from the anomalous set (i.e. either $P_2$ or $P_3$), mark the example as "Reject".
    \item Remove every training example marked "Reject" from $D$, producing $D^*$.
    \item Retrain on $D^*$, producing cleaned model $M^*$.
\end{enumerate}

\subsection{Extension: Test-time detection}

The algorithm in \ref{sec:algorithm} can be modified to permit test-time classification in the following way:

\begin{enumerate}
    \item Using a test set of data $D_T$, create clean and poisoned probes similarly to on the training set. 
    \item When training $M'$, store checkpoints of the model at each epoch.
    \item Once training has completed, save the loss-trajectories of the clean and poisoned \textit{test} probes as a k-nearest neighbors classifier.
    \item At test time, evaluate the test point on the sequence of checkpoints of $M'$.
    \item Use kNN classification using the test probe loss trajectories to determine whether the example is backdoored or not.
\end{enumerate}

\subsection{Additional Figures}

See: Figure~\ref{fig:loss_trajectories_cifar10}
\begin{figure}[t]
    \centering
    \begin{subfigure}[b]{0.66\textwidth}
         \centering
        \includegraphics[width=\textwidth]{Figures/trajectories/loss_trajectories_cifar10_cleaned.pdf}
        \caption{Loss trajectories}
    \end{subfigure}
    \begin{subfigure}[b]{0.326\textwidth}
         \centering
        \includegraphics[width=\textwidth]{Figures/trajectories/trajs_tsne.pdf}
        \caption{t-SNE embeddings}
    \end{subfigure}
    \caption{\textbf{Loss dynamics on CIFAR-10 with many simultaneous backdoor attacks} \citep{gu2017badnets, chen2017backdoor, nguyen2021wanet} (a) Visualization of the loss trajectories from the first 20 epochs. Fainted lines represent individual example trajectories while solid lines represent the mean trajectory. (b) t-SNE embeddings of the loss trajectories. The figure provides evidence that the training dynamics on backdoored examples are distinct from the clean examples without any backdoors.}
    \label{fig:loss_trajectories_cifar10}
\end{figure}

\subsection{Training details}
\label{sec:train-details}
\begin{itemize}
    \item Architecture: ResNet-50.
    \item Epochs: 100
    \item Batch Size: 128 (CIFAR-10), 256 (GTSRB)
    \item Optimizer: AdamW
    \item Learning rate: 1e-3
    \item Weight Decay: 1e-4
    \item LR Schedule: Cosine Annealment
    \item No augmentations
\end{itemize}
